# Supplementary material for: From glass formation to icosahedral ordering by curving three-dimensional space
Source: arXiv:1609.03044 ancillary file (2017-05-04)
Supplement: Supplementary file 1 [file LU15768-supplementary-resubmission-3rdApril2017.pdf]

## Supplementary Material

# From glass formation to icosahedral ordering by curving three-dimensional space

Francesco Turci,[1,*] Gilles Tarjus,[2] and C. Patrick Royall[1,3,4]

[1] *H.H. Wills Physics Laboratory, Tyndall Avenue, Bristol, BS8 1TL, UK*
[2] *LPTMC, CNRS-UMR 7600, Université Pierre et Marie Curie, boîte 121, 4 Pl. Jussieu, 75252 Paris cedex 05, France*
[3] *School of Chemistry, University of Bristol, Cantock's Close, Bristol, BS8 1TS, UK*
[4] *Centre for Nanoscience and Quantum Information, Tyndall Avenue, Bristol, BS8 1FD, UK*

### MODEL AND MONTE-CARLO SIMULATIONS ON $S^3$

The Wahnström binary mixture is composed of A and B particles interacting via a Lennard-Jones potential

$$u_{ij(r)} = 4\epsilon\left(\frac{\sigma_{ij}}{r^{12}} - \frac{\sigma_{ij}}{r^{6}}\right) \tag{1}$$

where $r$ is the geodesic distance on the 3-sphere $S^3$ , $\epsilon$ the energy scale, $\sigma_{AA} = \sigma_A = 1.2\sigma_{BB} = 1.2\sigma_B$ and $\sigma_{AB} = (\sigma_A + \sigma_B)/2$ are the diameters of interaction, with cutoff distance at $r_{cut} = 2.5\sigma_{ij}$ and masses $m_A/m_B, = 2.0$. Energy is measured in units of $\epsilon$ and lengths in $\sigma_A$. The Boltzmann factor $k_B$ is set to unity.

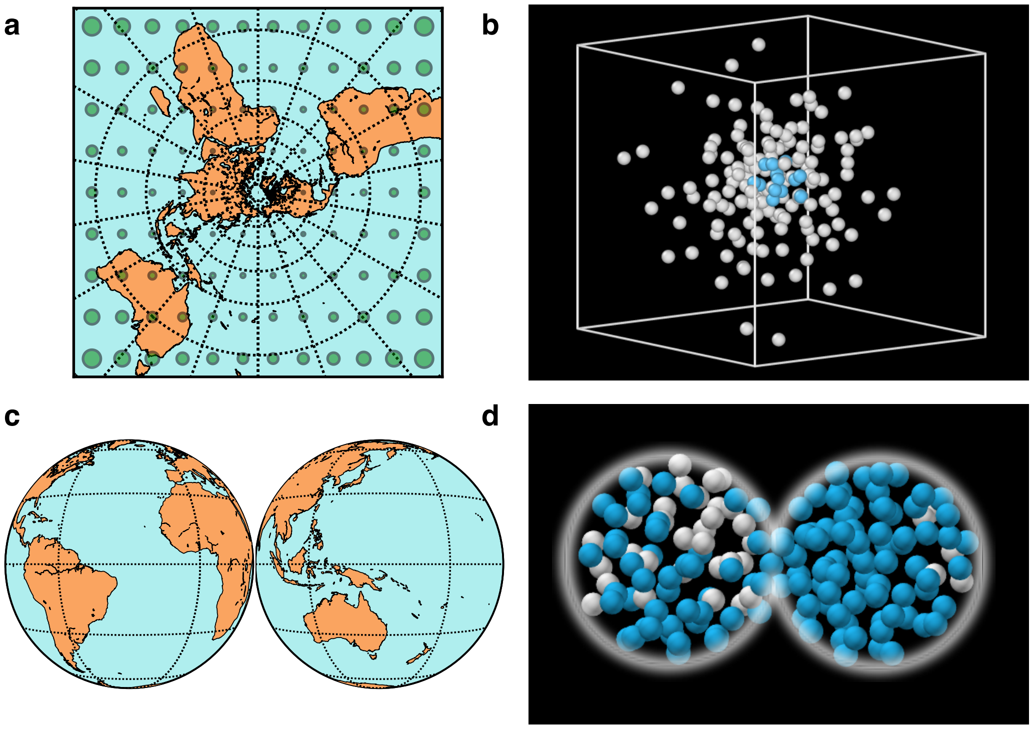


FIG. S1. (a) Stereographic projection of the Earth. Green circles demonstrate how distances and areas vary at larger and larger distances from the pole (also called *Tissot's indicatrix*). (b) Stereographic projection of the 3-sphere with $N = 240$ around a pole (where the Euclidean approximation is more valid). The particles are further and further apart when they are more and more distant from the pole. An icosahedral domain of particles is highlighted in blue. Two-balls construction for the Earth (as it would be seen by two geo-stationary satellites) (c) and the 3-sphere with $N = 160$ (d): the circumference in (c) or the spherical surfaces (white halo in (d)) are mapped to each other. An extended domain of particles in icosahedra is highlighted in blue.

We access the structure and the dynamics of the Wahnström binary mixture in curved three-dimensional space through Monte-Carlo simulations, in which particles perform random moves of maximum displacement $\Delta r_{\max} = 0.2\sigma_A$ that are accepted or rejected according to the Metropolis-Hastings algorithm. Time is measured in Monte-Carlo sweeps, where 1 sweep is equivalent to N attempts. Finally, time is rescaled according to the physics of the system: we choose the relaxation time $\tau(N)|_{T=3}$ obtained from the dynamic correlation functions at very high temperature $T = 3$ as a unit for all the computed relaxation times.

The displacements on $S^3$ are constructed following Marsaglia's method for the selection of points on a d-dimensional sphere [1], as improved and illustrated by Kratky and Schreiner [2]. This allows us to select displacements that are isotropic on the 3-sphere but not uniform in the interval $[0, \Delta r_{\max}]$, as they favor moves of order $\Delta r_{\max}$. Nonetheless, since $\Delta r_{\max} \ll \sigma_A$, the resulting sampling produces dynamics and equilibrium structures of the liquid that do not depend on the specific choice of $\Delta r_{\max}$. Depending on the system size and temperatures, $10^6$ to $10^7$ Monte-Carlo sweeps have been executed, for a maximum of 90 CPU hours.

To visualize the configurations on the surface of the 4-d hypersphere and monitor the growth of order, we have used projections. This surface is a compact 3-dimensional manifold with no border. Particle positions are identified by the vector $\vec{r} = (x, y, z, w)$, only 3 of which are independent.

A first possible projection is the stereographic projection, which maps the 3-sphere $S^3$ on $\mathbb{R}^3$. This consists in taking the following transformation

$$\vec{r} = (x, y, z, w) \in S^3 \to \left( \frac{x}{w-1}, \frac{y}{w-1}, \frac{z}{w-1} \right) \in \mathbb{R}^3 \tag{2}$$

The sphere is therefore mapped onto the 3-dimensional space, plus a point at infinity. This transformation does not preserve areas, and it therefore induces some distortions, which are illustrated more transparently in the case of the 2-sphere (see Figure S1 (a) where a stereographic projection of the Earth is represented). However, locally this transformation allows one to identify the relationships between neighboring particles: for instance, in Figure S1 (b) we observe an isolated icosahedral cluster for a system of $N = 240$ particles at temperature $T = 1.5$.

An alternative representation of the 3-sphere is the two-balls model (Figure S1 c and d). In this projection the particle coordinates are represented inside two 2-spheres (for positive and negative values of $w$ respectively) which share their respective surfaces (they are topologically *glued* together). This is analogous to splitting the surface of the Earth into two hemispheres (see Figure S1 c), represented as two circles, and imposing a mapping between the two circumferences. As a side note, this is a useful construction in order to have an intuitive sense of a 3-sphere surface, a closed 3-dimensional manifold that one can navigate without ever encountering any edge, in close relationship with modern relativistic cosmology and surprisingly analogous to the medieval model of the universe proposed by Dante in his *Commedia* [3].

## NEIGHBORS AND DYNAMIC CORRELATION FUNCTIONS

When identifying the network of (nearest) neighbors in liquids and disordered structures, Voronoi tessellations are commonly used in order to define the neighborhood of a particle in a nonambiguous way. It can be shown [4] that on spheres, the tessellation corresponds to the projection on the spherical surface of the convex hull of the set of points representing the centers of the particles. Under this projection, the simplexes of the convex hull correspond to the Voronoi cells.

In the present case, we consider the convex hull of the centers of the Wahnström binary mixture moving on the surface of the 3-sphere and analyze the simplexes, from which we obtain a list of neighbors for every particle. In order to take into account only nearest neighbors, we filter the neighbor lists to retain only particles that are within a distance $d_{\max}$ set by the first minimum of the equilibrium radial correlation function $g(r)$.

We identify for a given particle $i$ at time $t$ all its nearest neighbors and correspondingly construct and indicator vector $\vec{v}_i(t)$. The $j$-th element of vector $\vec{v}_i(t)$ takes value 1 if $i$ and $j$ are neighbors or 0 otherwise. With these definitions, we compute a time-correlation function

$$C(t) = \left\langle \frac{1}{N} \sum_{i=1}^{N} \frac{\vec{v}_i(t_0 + t) \cdot \vec{v}_i(t_0)}{\vec{v}_i^2(t_0)} \right\rangle_{t_0} . \tag{3}$$

$C(t)$ does not decay to zero in the long-time limit: this nonzero limit reflects the finite probability to find particle $i$ close to particle $j$ in a finite system of $N$ particles. We therefore fit $C(t)$ to a shifted stretched exponential form,

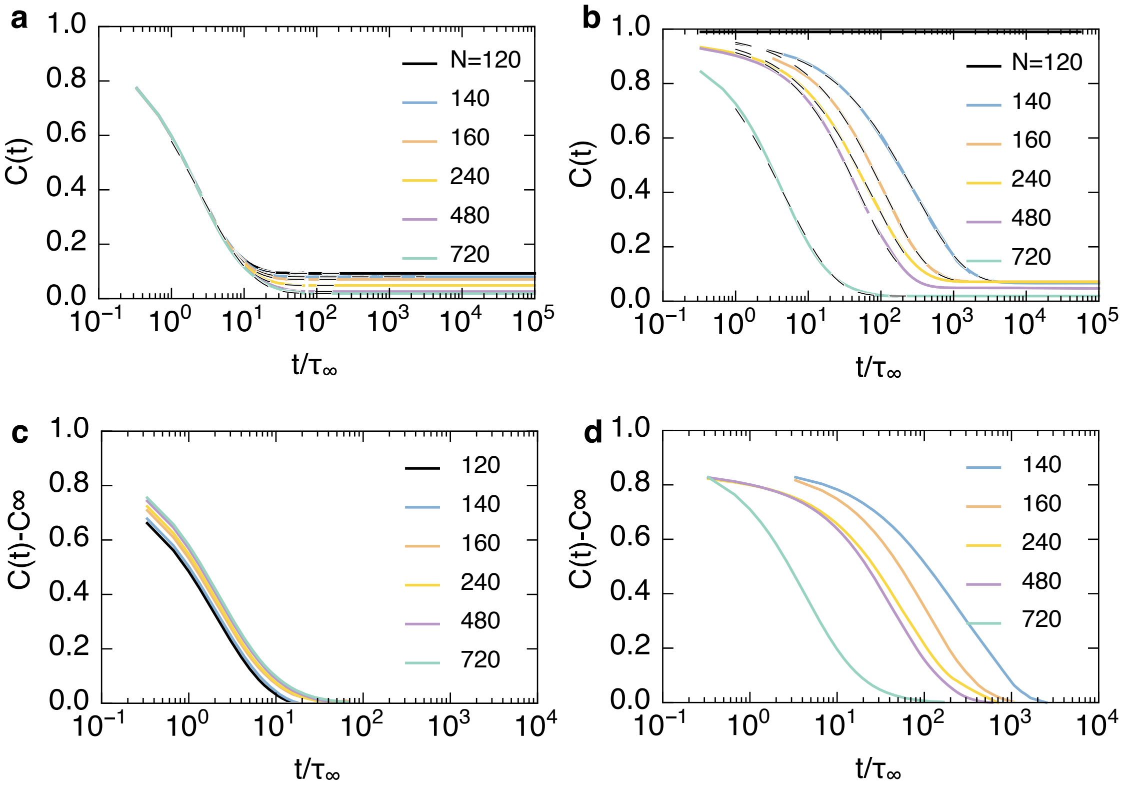


FIG. S2. Time-dependent correlation functions $C(t)$ at high temperature $T = 2$ (a) and lower temperature T=0.8 (b) for different curvatures (as indicated by the number of particles). Dashed lines indicate shifted stretched exponential fits. In (c) and (d) we show the same data for $C(t) - C(\infty)$, where $C(\infty) = \lim_{t\to\infty} C(t)$.

$C(t) = a + b\exp[-(t/\tau)^{\beta}]$, from which we extract the characteristic time for cage-breaking, *i.e.* the structural ($\alpha$) relaxation time $\tau$. This is illustrated in Figure S2.

## N=120 AND THE {3,3,5} POLYTOPE

For the curvature corresponding to $N = 120$ at sufficiently low temperatures, all the particles of the binary mixture are detected as participating to a network of icosahedra. This is compatible with a tessellation of the hypersphere according to the regular {3,3,5} polytope and the formation of a fully ordered phase is reminiscent of crystallization.

The final ordered state has a very reduced mobility (see main text). However, since the system is finite and is a binary mixture, fluctuations in the degree of local order may occur and defects in the icosahedral order can be present. To check this we have computed the coordination number $Z$ of each atom, *i.e.*, the number of nearest neighbors obtained from the Voronoi tesselation. The result is shown for temperatures ranging from $T = 3.0$ to the coldest temperature for this system size, $T = 0.8$ in Fig. S3 (a). We find that at the coldest temperature 96% of the atoms have 12 neighbors, which is compatible with the icosahedral environment. The remaining 5 or less atoms have 13 neighbors and can be considered in some sense as defects. It is unclear however if they can be described as topological defects in the form of disclination lines. Note also that the constraints on the average coordination number $\overline{Z}$ is not as strong in $d = 3$ as it is in $d = 2$ [5] and atomic assemblies on a 3-sphere with a curvature that is compatible with the {3,3,5} polytope need not have exactly $\overline{Z} = 12$.

Finally, we also observe that at very low temperatures the different interactions between the different particle types can lead to a partial separation of the particle types, as illustrated by the representation in Fig. S3(b). However, no complete segregation is observed.

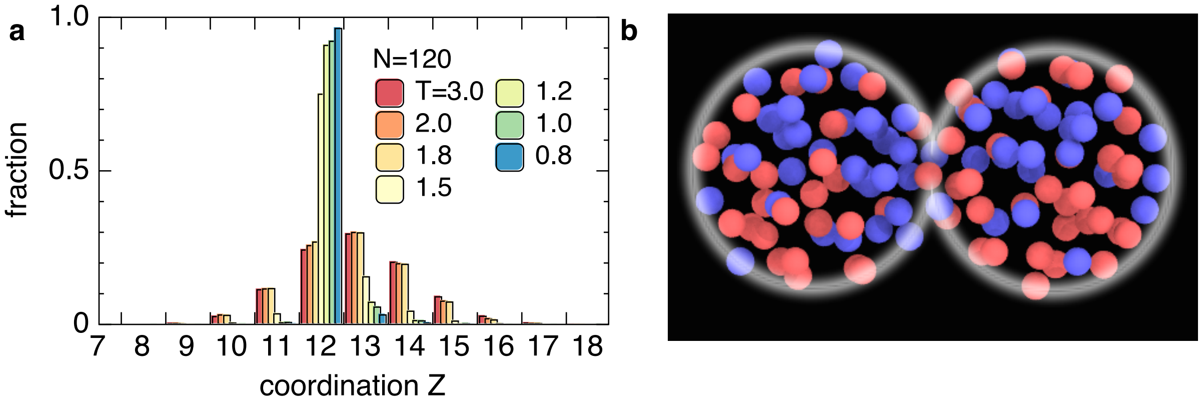


FIG. S3. Structure of the icosahedral phase for $N = 120$ (a) Histogram of the coordination number $Z$ of the 120 atoms for several temperatures. At the coldest temperature $T = 0.8$, Only 5 or less atoms do not have 12 neighbors as in an icosahedral environment. (b) Particles of type A (red) and particles of type B (blue) in the two-ball representation of $S^3$ at $T = 0.8$.

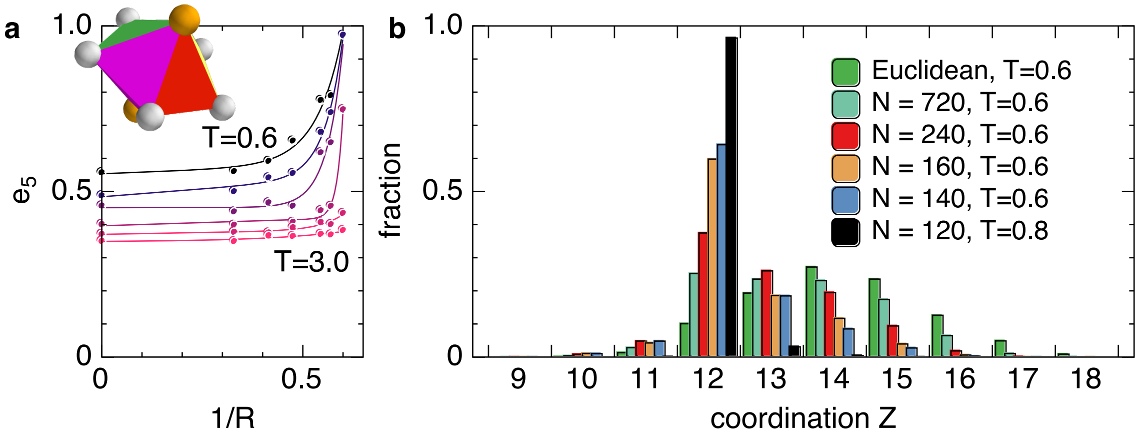


FIG. S4. (a) Fraction of bonds sharing 5 tetrahedra $e_5$ as a function of the inverse sphere radius $1/R$ for several temperatures $T = 0.6, 0.8, 1.0, 1.5, 2.0, 3.0$. Lines are guides for the eye. In the inset, two spindle particles (orange) form a bond which shares five coloured tetrahedra. (b) Histogram of the coordination number $Z$ for several values of $N$ at low temperature.

## VARIATION WITH CURVATURE OF THE STRUCTURE OF THE LOW-$T$ PHASE ON $S^3$

To characterize the progressive frustration of icosahedral order as curvature increases we have computed on top of the concentration of particles participating in icosahedral clusters (see Fig. 1 of the main text) two additional quantities: the fraction of bonds (defined in the Voronoi tesselation) sharing 5 tetrahedra and the histogram of coordination numbers (see above). We show the results as $N$ increases for different temperatures in Fig. S4. We see the same trend as for the concentration of atoms in icosahedral clusters. At the coldest temperature, the fraction of bonds sharing 5 tetrahedra rapidly decreases from almost 100% for $N = 120$ to 55% in the Euclidean space. Similarly the average coordination number at low $T$ $\overline{Z}$ increases from 12.04 for $N = 120$ at the coldest temperature $T = 0.8$ to 13.96 in the Euclidean space at temperature $T = 0.60$ and the histogram progressively broadens and.

We have also tested the possible emergence of a Frank-Kasper phase at curvature increases. (Recall that crystallization of the Wahnström binary mixture in Euclidean space takes place to such a phase [6].) In particular, we determine the particles associated to the Frank-Kasper bond through the identification in the Voronoi tessellation of all the motifs composed by a pair of A particles sharing 6 common B neighbours. We then compute the total number particles participating to such motifs $N_{FK}$ and the corresponding fraction $n_{FK} = N_{FK}/N$ as a function of curvature and temperature. As seen from Fig. S5, this fraction remains small and almost constant for the strongest curvatures. In particular, for $N = 120$ the fraction of particles in Frank-Kasper bonds vanishes as the system crystallises. It is then moderately depleted in the ordered phase of $N = 120, 160$, almost constant for $N = 240$ and it shows a moderate increase for the lowest curvatures accessible to our simulations. This becomes a stronger increase rate in the Euclidean

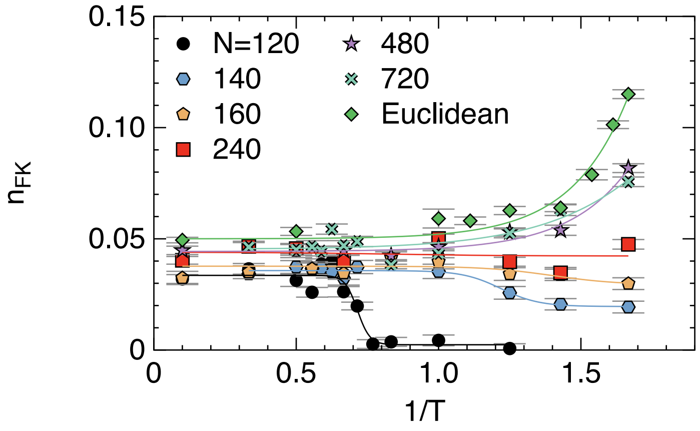


FIG. S5. Fraction $n_{FK}$ of particles participating to the 2A-6B Frank-Kasper motif for different $N$ and temperatures $T$. Lines are guides for the eye.

case, as initially observed by Pedersen *et al.* [6]. This suggests that, for the corresponding curvature, the increase of icosahedral order at a given temperature with respect to the Euclidean case occurs within an amorphous phase. It is possible that, as predicted by the geometric-frustration approach, crystallization to some form of Frank-Kasper phase takes place at a still lower temperature, but this would not change the interpretation of the liquid branch that undergoes a glass transition. However, we observe that, as the curvature is reduced, Frank-Kasper motifs play a more important role at low temperatures. This is compatible with our interpretation of the decoupling between static and dynamic lenthscales, in the main text, for which as frustration increases additional mechanisms come to play a role in the glass-forming ability of the system, with only remnants of the role of icosahedral ordering. One of such mechanisms could be the formation of the complex Frank-Kasper unit cell.

## DYNAMICAL AND STRUCTURAL LENGTHS

Dynamical and structural lengths are extracted in real space from the radial distribution functions of the particles detected as slow at time $t = \tau$ and from the particles forming icosahedral domains respectively. To do so, we fit the peaks of the radial distribution functions with the following functional form,

$$g_x^{\text{peaks}}(r) = A\frac{\exp(-r/\xi)}{r} + c \tag{4}$$

where $\text{x} = \text{slow}, \text{icos}$ respectively and $A, \xi, c$ are fitting constants. This form assumes that the correlations decay following the Ornstein-Zernike form of liquid state theory [7].

Best fit lines are obtained by minimizing the deviations between the peak values of $|g_x(r) - c|$ and Eq. (4) as represented in Fig. S6.

From the fits, we obtain static and dynamic length scales $\xi_{\text{slow}}$ and $\xi_{\text{icos}}$. Both increase as a function of the inverse temperature, but with very different rates according to the curvature of $S^3$. As shown in Fig. S7, high curvatures (and small N) correspond to a very rapid increase of the icosahedral correlation length, while for $N \geq 240$ it has a more limited dynamic range. The dynamical length on the other hand has a non-monotonic variation with curvature of its rate of change with temperature (see Fig. 3 of the main text) with a minimum rate observed for $N = 240$ (among the values we have studied). For $N \geq 240$ one therefore finds that the temperature change of the dynamical length decouples more and more with that of the structural length, as illustrated in Fig. 3(c) of the main text.

## DYNAMICAL SUSCEPTIBILITY

As indicated in the main text, we measure the dynamical susceptibility $\chi(t)$

$$\chi(t) = \frac{1}{N}(\langle N_{\text{slow}}^2(t)\rangle - \langle N_{\text{slow}}(t)\rangle^2), \tag{5}$$

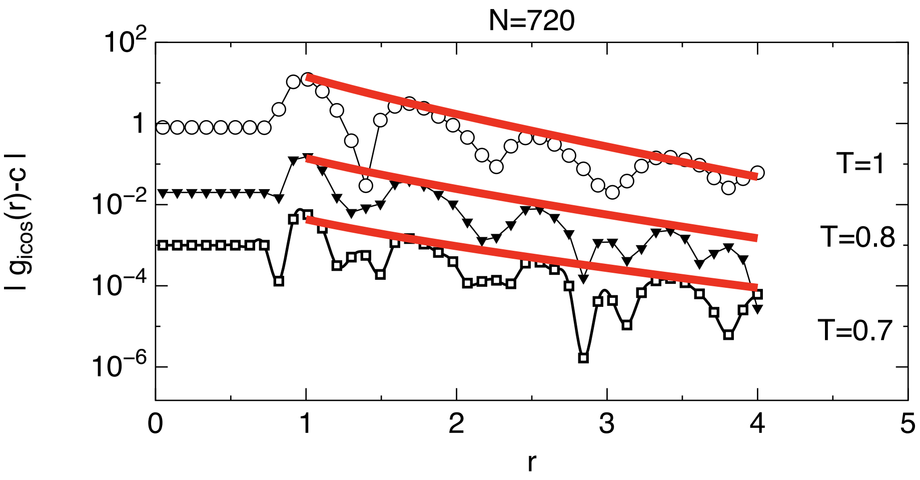


FIG. S6. Best fit curves (red straight lines) of the peaks of the radial distribution functions of icosahedral domains on the 3-sphere.

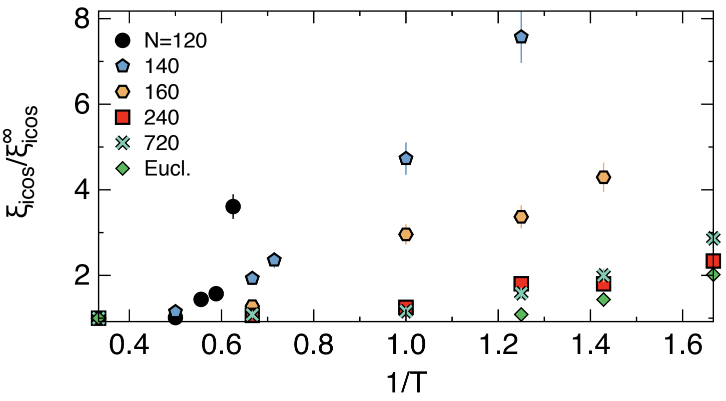


FIG. S7. Structural length (rescaled to its high-$T$ value) as a function of the inverse temperature for several system sizes $N$ corresponding to different curvatures.

where $N_{\text{slow}}$ is the number of slow particles at time $t$ (see main text). From its peak value we obtain an estimate of the size of the dynamically correlated regions, see Fig. S8, and observe that the smallest systems ($N = 120, 140$) present fast growing correlations upon cooling compared to the smaller curvature ones. (This occurs in the vicinity of the temperatures at which the high curvature systems access the icosahedral state.) The rate of change with decreasing temperature appears to be weakly non-monotonic, with a minimum variation for $N = 240$: see Fig. S9. This is in line with the result found for the dynamical length (see Fig. 3 of the main text and the discussion above).

* Corresponding author: f.turci@bristol.ac.uk

[1] G. Marsaglia, The Annals of Mathematical Statistics **43**, 645 (1972).
[2] K. W. Kratky and W. Schreiner, Journal of Computational Physics **47**, 313 (1982).
[3] M. A. Peterson, American Journal of Physics **47**, 1031 (1979).
[4] K. Sugihara, Journal for Geometry and Graphics **6**, 69 (2002).
[5] J.-F. Sadoc and R. Mosseri, *Geometrical frustration* (Cambridge University Press, 2006).
[6] U. R. Pedersen, T. B. Schroder, J. C. Dyre, and P. Harrowell, Phys. Rev. Lett. **104**, 105701 (2010).
[7] J.-P. Hansen and I. R. McDonald, *Theory of Simple Liquids: With Applications to Soft Matter* (Academic Press, 2013).

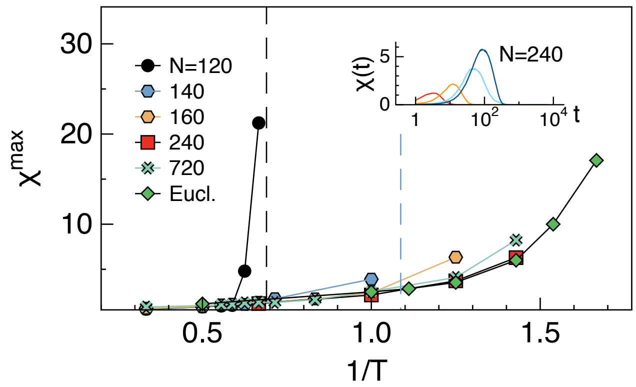


FIG. S8. Measure of the dynamical spatial correlations $\chi^{max}$: As illustrated in the inset, we extract the peak of $\chi(t)$ for different curvatures and temperatures. For the two smallest systems ($N = 120, 140$), the dynamics is inaccessibly slow below the vertical dashed lines and $\chi^{\max}$ is then virtually zero. In the Inset, $T = 1.5, 1, 0.8, 0.7$.

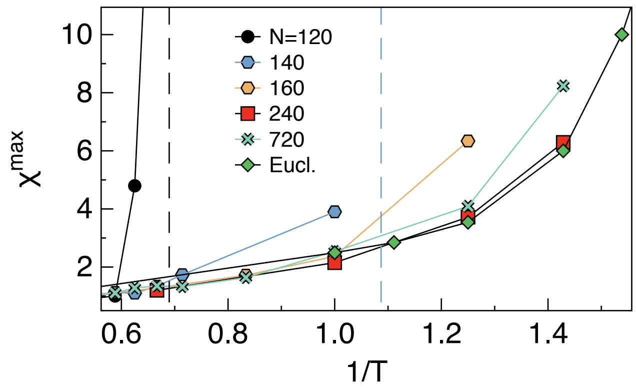


FIG. S9. Zoom in on the data in Fig. S8: The rate of change with decreasing $T$ seems to display a weak non-monotonic behavior as a function of curvature, with the smallest rate found for $N = 240$.
